# Supplementary material for: Antiferroelectric instability in kagome francisites Cu$_3$Bi(SeO$_3$)$_2$O$_2$X (X = Cl, Br)
Source: arXiv:1611.03317 ancillary file (2016-11-10)
Supplement: Supplementary file 1 [file francisite-structure-supplement.pdf]

# *Supplemental Material*

# Antiferroelectric instability in kagome francisites $Cu_3Bi(SeO_3)_2O_2X$ (X = Cl, Br)

Danil A. Prishchenko,[1] Alexander A. Tsirlin,[1,2] Vladimir Tsurkan,[3,4]
Alois Loidl,[3] Anton Jesche,[2] and Vladimir G. Mazurenko[1]

[1] *Ural Federal University, Mira Str. 19, 620002 Ekaterinburg, Russia*
[2] *Experimental Physics VI, Center for Electronic Correlations and Magnetism, Institute of Physics, University of Augsburg, 86135 Augsburg, Germany*
[3] *Experimental Physics V, Center for Electronic Correlations and Magnetism, Institute of Physics, University of Augsburg, 86135 Augsburg, Germany*
[4] *Institute of Applied Physics, Academy of Sciences Moldova, Chisinau MD-2028, Republic of Moldova*

This Supplemental material contains representative results of crystal structure refinement. The data were collected at the ID22 beamline of the ESRF using the wavelength of 0.41 Å. The refined crystal structures are provided as cif-files along with this Supplemental material.

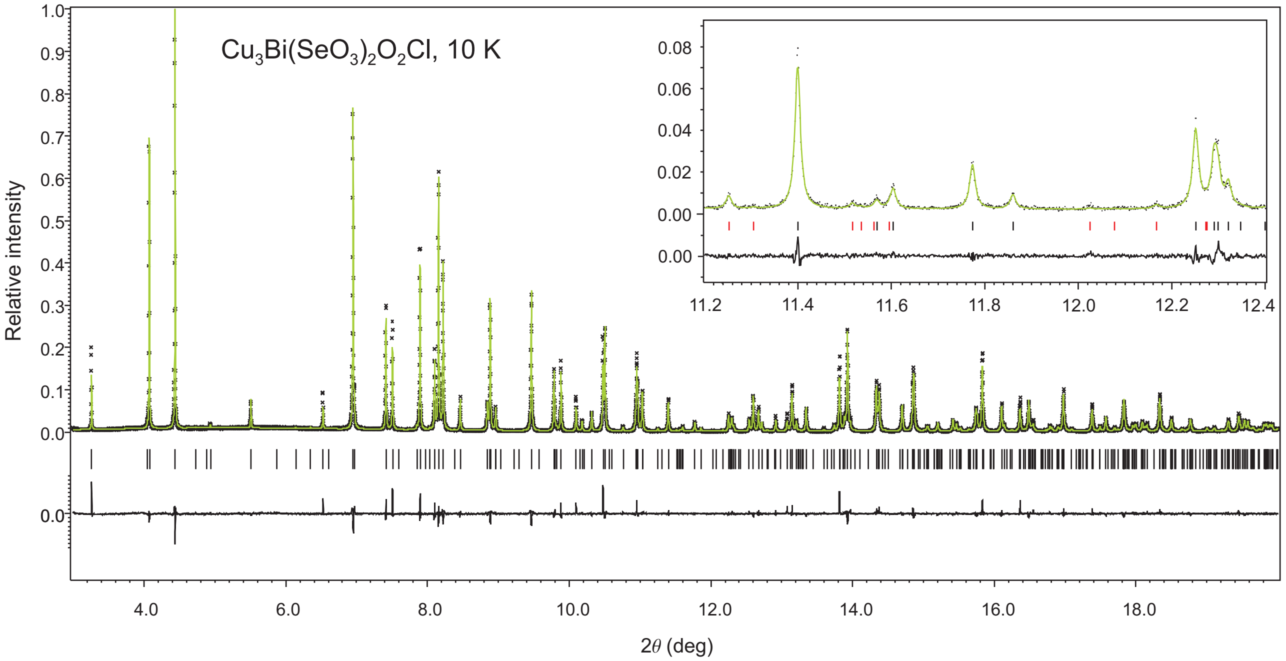


FIG. S1. X-ray structure refinement for $Cu_3Bi(SeO_3)_2O_2Cl$ at 10 K. Tick marks show reflection positions. The difference curve is in the bottom. The inset magnifies the angular range where the most intense superstructure reflections are observed. These reflections ($hkl$, $l=$odd) are labeled in red.

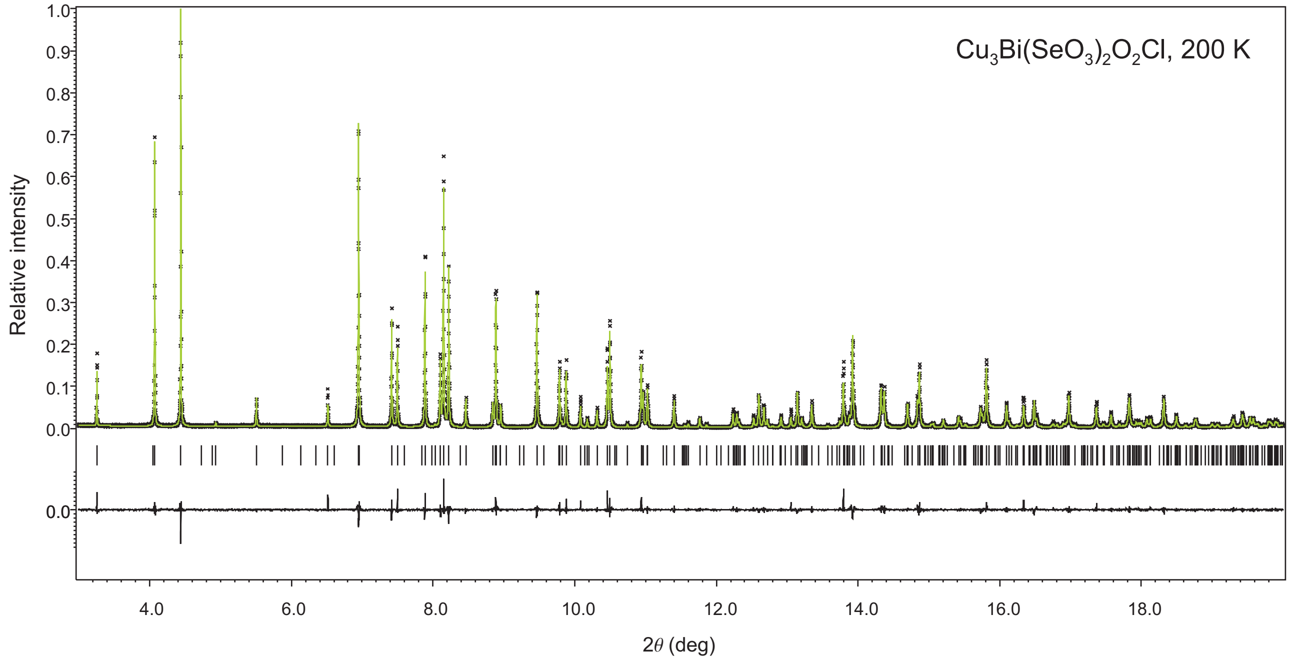


FIG. S2. X-ray structure refinement for $Cu_3Bi(SeO_3)_2O_2Cl$ at 200 K. Tick marks show reflection positions. The difference curve is in the bottom.

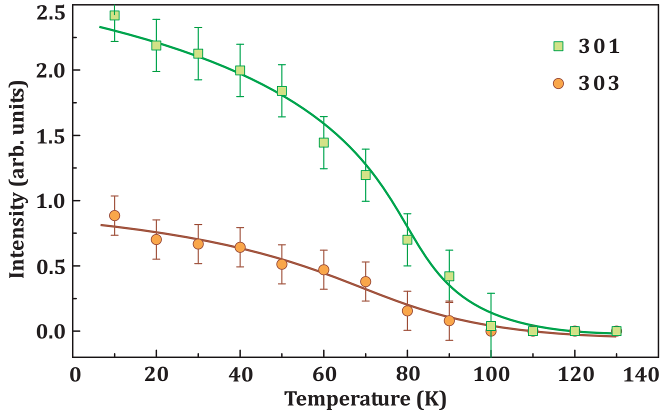


FIG. S3. Intensities of superstructure reflections 3 0 1 and 3 0 3 in $Cu_3Bi(SeO_3)_2O_2Cl$ as a function of temperature. The lines are guide-for-the-eye only.

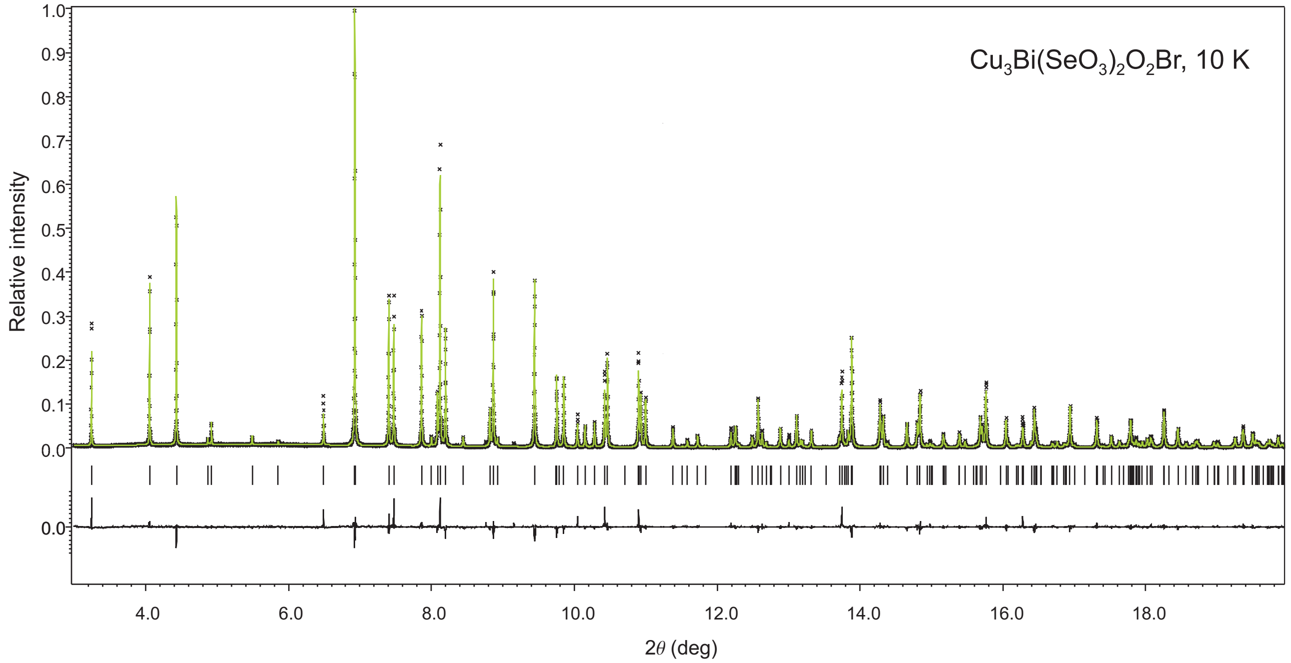


FIG. S4. X-ray structure refinement for $Cu_3Bi(SeO_3)_2O_2Br$ at 10 K. Tick marks show reflection positions. The difference curve is in the bottom.

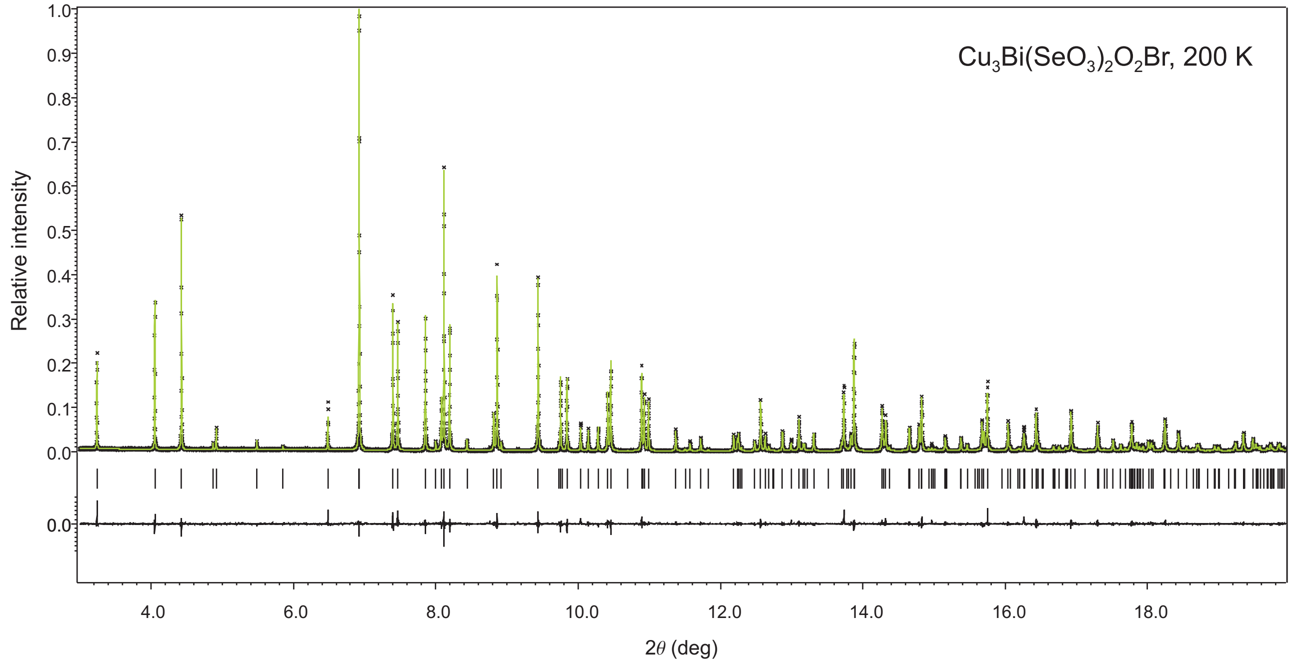


FIG. S5. X-ray structure refinement for $Cu_3Bi(SeO_3)_2O_2Br$ at 200 K. Tick marks show reflection positions. The difference curve is in the bottom.
